# Supplementary material for: Approximate Collapsed Gibbs Clustering with Expectation Propagation
Source: arXiv:1807.07621 source file (2018-07-19)
Supplement: Supplementary file 1 [file supp_scalemix.tex]

This section provides the supplementary material for
Sec.~\ref{sec:scalemix} on Gaussian scale mixtures (GSM).
We provide the details on how to calculate the sufficient statistics of
$\mu, \Sigma$ required for our EP approximation.

We now present how to collapse out $\mu, \Sigma$,
approximating $p(\mu, \Sigma | y, z, w,r)$ with a normal inverse-Wishart.

This consists of estimating three quantities from the tilted distribution
(i) the normalizing constant $\tilde{Z}_i$,
(ii) the mean $\E_{\tilde{p}_i}[\mu]$, and
(iii) the second moment $\E_{\tilde{p}_i}[\mu \mu^T]$.

The normalizing constant (a.k.a. the likelihood approximation) is a weighted
average
\begin{equation}
    \tilde{Z}_i = 
    \int f(y_i \,  \, \mu, \Sigma, w) q(\mu \, | \, z_{-i}) \ d \mu
    = 
    \sum_{c = 1}^C \int w_c \cdot \mathcal{N}(y_i \, | \, \mu,\Sigma_c)
    \cdot \mathcal{N}(\mu \, | \, \mu_{-i}, \Sigma_{-i}) \ d\mu 
    =
    \sum_{c = 1}^C w_c \cdot \tilde{Z}_c 
    \enspace,
\end{equation}
where $\tilde{Z}_c$ is the normalizing constant treating only component $c$
as likelihood.
This is easy t do since component $c$ is a Gaussian, which is conjugate.

Similarly, the tilted-mean and second moments are weighted averages
\begin{align}
    \nonumber
    \E_{\tilde{p}_i}[\mu] &= 
    \int \mu \cdot \tilde{Z}_i^{-1} f(y_i \, | \, \mu, \Sigma, w)
    q(\mu \, | \, z_{-i}) \ d \mu 
    \\ \nonumber &=
    \sum_{c = 1}^C \frac{w_c \tilde{Z}_c}{\tilde{Z}_i} \int 
    \mu \cdot \underbrace{
        \tilde{Z}_c^{-1} \mathcal{N}(y_i \, | \, \mu,\Sigma_c)
        \cdot \mathcal{N}(\mu \, | \, \mu_{-i}, \Sigma_{-i})
    }_{\tilde{p}_c(\mu)} \ d\mu 
    \\ &=
    \sum_{c = 1}^C \frac{w_c \tilde{Z}_c}{\tilde{Z}_i} \, \E_{\tilde{p}_c}[\mu]
\end{align}
\begin{align}
    \nonumber
    \E_{\tilde{p}_i}[\mu \mu^T] &= 
    \int \mu\mu^T \cdot \tilde{Z}_i^{-1} f(y_i \, | \, \mu, \Sigma, w)
    q(\mu \, | \, z_{-i}) \ d \mu 
    \\ \nonumber &=
    \sum_{c = 1}^C \frac{w_c \tilde{Z}_c}{\tilde{Z}_i} \int 
    \mu\mu^T \cdot \underbrace{
        \tilde{Z}_c^{-1} \mathcal{N}(y_i \, | \, \mu,\Sigma_c)
        \cdot \mathcal{N}(\mu \, | \, \mu_{-i},\Sigma_{-i})
    }_{\tilde{p}_c(\mu)} \ d\mu 
    \\ &=
    \sum_{c = 1}^C \frac{w_c \tilde{Z}_c}{\tilde{Z}_i} \, 
    \E_{\tilde{p}_c}[\mu\mu^T] \enspace,
\end{align}
where $\tilde{p_c}$ is the posterior for $\mu$ treating only component $c$ as
the likelihood.
